# Supplementary material for: FedCore: Straggler-Free Federated Learning with Distributed Coresets
Source: arXiv:2402.00219 source file (2024-01-31)
Supplement: Supplementary file 1 [file algorithm.tex]

\section{Detailed Algorithm of \name{}}\label{sec:apend_algo}

\begin{algorithm}[ht]
\begin{algorithmic}[1]
\footnotesize
    \caption{\name{} Algorithm}
    \label{alg:fedcore}	
    \STATE {\bf Input:}  $K$, $T$, $w_0$, $E$, $\tau$, and $V^i$, $c^i$, $m^i$ for all $i\in U$\\
           {~~~~~~~~~~~} $E$, $\tau$, and $V^i$, $c^i$, $m^i$ for all $i\in U$ as they are defined in \cref{sec:preliminaries}
    \FOR  {$t=1, \cdots, T$}
        \STATE Server selects a subset of K clients $U_t \subseteq U$ at random. Each device $i$ is chosen\\
        with probability proportional to their training set size, i.e., {\small $p_i = \frac{m^i}{\sum_{i \in U}m^i}$}
        \FOR {\textbf{each} $i \in U_t$}
            \STATE Server sends $w_t$ to each chosen client        
            \IF {$E\cdot m^i < c^i\tau$}
                \STATE Train $E$ epochs of SGD algorithm over the entire dataset $V^i$
            \ELSE
                \STATE Trains one epoch over the entire training set $V^i$, and generates $\widetilde{d}^i_{j,k}$ or $\widehat{d}^i_{j,k}$ \\
                for different types of machine learning models (\cref{subsec:gradient_approx})
                \STATE Generates training coreset $(S^i, \delta^i)$ by solving the k-medoids problem Eq.\eqref{eq:opt_medoids}
                \STATE Trains $E-1$ epochs over the coreset $(S^i, \delta^i)$
            \ENDIF
            \STATE Each client $i \in U_t$ sends its local model parameter $w^i_{t+1}$ back to the server
        \ENDFOR
        \STATE Server aggregates the $w$'s as
        {\small $w_{t+1} = \frac{1}{K}\sum_{i \in U_t} w^i_{t+1}$}
    \ENDFOR
\end{algorithmic}
\end{algorithm}
